# Supplementary material for: Semi-Supervised Safe Visuomotor Policy Synthesis using Barrier Certificates
Source: arXiv:2409.12616 source file (2024-09-19)
Supplement: Supplementary file 1 [file Appendix.tex]

\begin{appendices}

\section{Proof of Theorem \ref{thm: Dynamics Guarantees}}

\end{appendices}
